# Supplementary material for: ReFine: Boosting Time Series Prediction of Extreme Events by Reweighting and Fine-tuning
Source: arXiv:2409.14232 source file (2024-09-21)
Supplement: Supplementary file 1 [file 7_appendix.tex]

\onecolumn
